# Supplementary material for: Towards Driving Policies with Personality: Modeling Behavior and Style in Risky Scenarios via Data Collection in Virtual Reality
Source: arXiv:2303.04901 source file (2023-03-08)
Supplement: Supplementary file 1 [file additionaldemographics.tex]

\centering
\begin{tabular}{llr}
\toprule
Gender & Male &  60\% \\
          & Female &  35\% \\
          & Non-binary &   5\% \\
Ethnicity & Asian &  60\% \\
          & Black/African &  10\% \\
          & Caucasian & 20\% \\
          & Armenian/Jewish & 5\% \\
          & South East Asian & 5\% \\
Age group & 18-29 &  90\% \\
          & 30-45 &  10\% \\
% Role & Undergraduate student &  60\% \\
%           & Graduate student &  40\% \\
\bottomrule
\end{tabular}
\label{tab:demographics}
